# Supplementary material for: Physics to the Rescue: Deep Non-line-of-sight Reconstruction for High-speed Imaging
Source: arXiv:2205.01679 source file (2022-08-06)
Supplement: Supplementary file 1 [file 07_supplementary.tex]

\begin{table}[]
\begin{tabular}{c||ccc}
\hline
\multirow{2}{*}{Method} & \multicolumn{3}{c}{Alphanumerics}                 \\ \cline{2-4} 
                        & RMSE           & PSNR            & SSIM           \\ \hline\hline
RSD                     & 0.084          & 22.023          & 0.395          \\
LFE                     & 0.064          & 24.335          & 0.886          \\
NeTF                    & 0.087          & 21.835            & 0.895          \\
NeTF++                  & 0.083          & 21.835          & 0.895          \\ \hline
Ours (\textit{sup})              & 0.059          & 24.936          & \textbf{0.905} \\
Ours (\textit{unsup})           & 0.073          & 23.124          & 0.833          \\
Ours (\textit{joint})            & \textbf{0.057} & \textbf{25.154} & 0.896          \\ \hline
\end{tabular}
\end{table}

\begin{table}[]
\begin{tabular}{c||ccc}
\hline
\multirow{2}{*}{Method} & \multicolumn{3}{c}{CMU} \\ \cline{2-4} 
                        & RMSE   & PSNR   & SSIM  \\ \hline\hline
RSD                     & 0.086  & 21.535 & 0.456 \\
LFE                     & 0.082  & 21.835 & 0.700 \\
NeTF                    & 0.100  & 20.312 & 0.795 \\
NeTF++                  & 0.071  & 23.263 & 0.815 \\ \hline
Ours (\textit{sup})             & 0.076  & 22.463 & 0.799 \\
Ours (\textit{unsup})           & 0.070  & 23.181 & 0.775 \\
Ours (\textit{joint})                & 0.079  & 22.107 & 0.798 \\ \hline
\end{tabular}
\end{table}

% fused table without RSD and IFE
\begin{table}[]
\begin{tabular}{c||ccc|ccc}
\hline
                         & \multicolumn{3}{c|}{\cellcolor[HTML]{FFFFFF}Alphanumerics} & \multicolumn{3}{c}{\cellcolor[HTML]{FFFFFF}CMU} \\ \cline{2-7} 
\multirow{-2}{*}{Method} & RMSE              & PSNR               & SSIM              & RMSE           & PSNR           & SSIM          \\ \hline \hline
NeTF                     & 0.087             & 21.993             & 0.893             & 0.100            & 20.312         & 0.795         \\
NeTF++                   & 0.083             & 21.835             & 0.895             & 0.071          & 23.263         & 0.815         \\ \hline
Ours (\textit{sup})               & 0.059             & 24.936             & 0.905             & 0.076          & 22.463         & 0.799         \\
Ours (\textit{unsup})             & 0.073             & 23.124             & 0.833             & 0.070           & 23.181         & 0.775         \\
Ours (\textit{joint})             & 0.057             & 25.154             & 0.896             & 0.079          & 22.107         & 0.798         \\ \hline
\end{tabular}
\end{table}

%fused table with RSD and LFE
\begin{table}[]
\begin{tabular}{c||ccc|ccc}
\hline
\multirow{2}{*}{Method} & \multicolumn{3}{c|}{Alphanumerics} & \multicolumn{3}{c}{CMU} \\ \cline{2-7} 
                        & RMSE      & PSNR       & SSIM      & RMSE   & PSNR   & SSIM  \\ \hline \hline
RSD                     & 0.084     & 22.023     & 0.395     & 0.086  & 21.535 & 0.456 \\
LFE                     & 0.064     & 24.335     & 0.886     & 0.082  & 21.835 & 0.700 \\
NeTF                    & 0.087     & 21.993     & 0.893     & 0.100  & 20.312 & 0.795 \\
NeTF++                  & 0.083     & 21.835     & 0.895     & 0.071  & 23.263 & 0.815 \\ \hline
Ours (\textit{sup})     & 0.059     & 24.936     & 0.905     & 0.076  & 22.463 & 0.799 \\
Ours (\textit{unsup})   & 0.073     & 23.124     & 0.833     & 0.070  & 23.181 & 0.775 \\
Ours (\textit{joint})   & 0.057     & 25.154     & 0.896     & 0.079  & 22.107 & 0.798 \\ \hline
\end{tabular}
\end{table}

\begin{sidewaystable}[]

\begin{minipage}{0.45\textwidth}
\centering

\begin{tabular}{c|ccccccccccccccccccccc}
\hline
 &
  \multicolumn{21}{c|}{\cellcolor[HTML]{FFFFFF}alphanumerics} \\ \cline{2-22} 
 &
  \multicolumn{3}{c|}{RSD} &
  \multicolumn{3}{c|}{LFE} &
  \multicolumn{3}{c|}{NeTF} &
  \multicolumn{3}{c|}{NeTF++} &
  \multicolumn{3}{c|}{Ours (sup)} &
  \multicolumn{3}{c|}{Ours (unsup)} &
  \multicolumn{3}{c}{Ours (joint)} \\ \cline{2-22} 
 &
  RMSE &
  PSNR &
  \multicolumn{1}{c|}{SSIM} &
  RMSE &
  PSNR &
  \multicolumn{1}{c|}{SSIM} &
  RMSE &
  PSNR &
  \multicolumn{1}{c|}{SSIM} &
  RMSE &
  PSNR &
  \multicolumn{1}{c|}{SSIM} &
  RMSE &
  PSNR &
  \multicolumn{1}{c|}{SSIM} &
  RMSE &
  PSNR &
  \multicolumn{1}{c|}{SSIM} &
  RMSE &
  PSNR &
  SSIM \\ \hline
9 &
  0.075 &
  22.538 &
  \multicolumn{1}{c|}{0.299} &
  0.056 &
  24.992 &
  \multicolumn{1}{c|}{0.896} &
  0.085 &
  21.435 &
  \multicolumn{1}{c|}{0.924} &
  0.075 &
  22.546 &
  \multicolumn{1}{c|}{0.935} &
  0.059 &
  24.609 &
  \multicolumn{1}{c|}{0.934} &
  0.077 &
  22.264 &
  \multicolumn{1}{c|}{0.881} &
  0.048 &
  26.428 &
  0.926 \\
lambda &
  0.050 &
  25.979 &
  \multicolumn{1}{c|}{0.519} &
  0.041 &
  27.694 &
  \multicolumn{1}{c|}{0.947} &
  0.041 &
  27.831 &
  \multicolumn{1}{c|}{0.972} &
  0.057 &
  24.878 &
  \multicolumn{1}{c|}{0.956} &
  0.039 &
  28.288 &
  \multicolumn{1}{c|}{0.963} &
  0.043 &
  27.389 &
  \multicolumn{1}{c|}{0.897} &
  0.040 &
  27.879 &
  0.944 \\
m &
  0.126 &
  18.014 &
  \multicolumn{1}{c|}{0.414} &
  0.085 &
  21.380 &
  \multicolumn{1}{c|}{0.811} &
  0.119 &
  18.506 &
  \multicolumn{1}{c|}{0.771} &
  0.096 &
  20.343 &
  \multicolumn{1}{c|}{0.795} &
  0.081 &
  21.877 &
  \multicolumn{1}{c|}{0.823} &
  0.086 &
  21.268 &
  \multicolumn{1}{c|}{0.758} &
  0.071 &
  22.946 &
  0.816 \\
mu &
  0.064 &
  23.862 &
  \multicolumn{1}{c|}{0.403} &
  0.048 &
  26.439 &
  \multicolumn{1}{c|}{0.928} &
  0.055 &
  25.261 &
  \multicolumn{1}{c|}{0.954} &
  0.080 &
  21.982 &
  \multicolumn{1}{c|}{0.932} &
  0.042 &
  27.588 &
  \multicolumn{1}{c|}{0.953} &
  0.058 &
  24.736 &
  \multicolumn{1}{c|}{0.896} &
  0.046 &
  26.774 &
  0.926 \\
sigma &
  0.067 &
  23.497 &
  \multicolumn{1}{c|}{0.456} &
  0.056 &
  25.045 &
  \multicolumn{1}{c|}{0.915} &
  0.078 &
  22.151 &
  \multicolumn{1}{c|}{0.927} &
  0.084 &
  21.548 &
  \multicolumn{1}{c|}{0.924} &
  0.054 &
  25.365 &
  \multicolumn{1}{c|}{0.931} &
  0.064 &
  23.816 &
  \multicolumn{1}{c|}{0.863} &
  0.054 &
  25.426 &
  0.929 \\
u &
  0.122 &
  18.249 &
  \multicolumn{1}{c|}{0.281} &
  0.095 &
  20.461 &
  \multicolumn{1}{c|}{0.821} &
  0.145 &
  16.775 &
  \multicolumn{1}{c|}{0.811} &
  0.103 &
  19.713 &
  \multicolumn{1}{c|}{0.828} &
  0.080 &
  21.890 &
  \multicolumn{1}{c|}{0.826} &
  0.109 &
  19.269 &
  \multicolumn{1}{c|}{0.703} &
  0.084 &
  21.473 &
  0.833 \\ \hline
average &
  0.084 &
  22.023 &
  \multicolumn{1}{c|}{0.395} &
  0.064 &
  24.335 &
  \multicolumn{1}{c|}{0.886} &
  0.087 &
  21.993 &
  \multicolumn{1}{c|}{0.893} &
  0.083 &
  21.835 &
  \multicolumn{1}{c|}{0.895} &
  0.059 &
  24.936 &
  \multicolumn{1}{c|}{0.905} &
  0.073 &
  23.124 &
  \multicolumn{1}{c|}{0.833} &
  0.057 &
  25.154 &
  0.896
\end{tabular}

\end{minipage}

\vspace{2cm}

\begin{minipage}{0.45\linewidth}
\centering

\begin{tabular}{l|ccccccccccccccccccccc}
\hline
 &
  \multicolumn{21}{c}{CMU} \\ \cline{2-22} 
 &
  \multicolumn{3}{c|}{RSD} &
  \multicolumn{3}{c|}{LFE} &
  \multicolumn{3}{c|}{NeTF} &
  \multicolumn{3}{c|}{NeTF++} &
  \multicolumn{3}{c|}{Ours (sup)} &
  \multicolumn{3}{c|}{Ours (unsup)} &
  \multicolumn{3}{c}{Ours (joint)} \\ \cline{5-22} 
 &
  RMSE &
  PSNR &
  \multicolumn{1}{c|}{SSIM} &
  RMSE &
  PSNR &
  \multicolumn{1}{c|}{SSIM} &
  RMSE &
  PSNR &
  \multicolumn{1}{c|}{SSIM} &
  RMSE &
  PSNR &
  \multicolumn{1}{c|}{SSIM} &
  RMSE &
  PSNR &
  \multicolumn{1}{c|}{SSIM} &
  RMSE &
  PSNR &
  \multicolumn{1}{c|}{SSIM} &
  RMSE &
  PSNR &
  SSIM \\ \hline
armadillo &
  0.060 &
  24.403 &
  \multicolumn{1}{c|}{0.361} &
  0.076 &
  22.393 &
  \multicolumn{1}{c|}{0.800} &
  0.067 &
  23.442 &
  \multicolumn{1}{c|}{0.815} &
  0.058 &
  24.686 &
  \multicolumn{1}{c|}{0.851} &
  0.066 &
  23.584 &
  \multicolumn{1}{c|}{0.843} &
  0.072 &
  22.804 &
  \multicolumn{1}{c|}{0.778} &
  0.065 &
  23.763 &
  0.823 \\
bear &
  0.089 &
  21.006 &
  \multicolumn{1}{c|}{0.539} &
  0.096 &
  20.322 &
  \multicolumn{1}{c|}{0.540} &
  0.101 &
  19.917 &
  \multicolumn{1}{c|}{0.771} &
  0.062 &
  24.163 &
  \multicolumn{1}{c|}{0.810} &
  0.073 &
  22.787 &
  \multicolumn{1}{c|}{0.748} &
  0.083 &
  21.582 &
  \multicolumn{1}{c|}{0.725} &
  0.078 &
  22.121 &
  0.792 \\
bunny &
  0.078 &
  22.121 &
  \multicolumn{1}{c|}{0.633} &
  0.059 &
  24.543 &
  \multicolumn{1}{c|}{0.739} &
  0.104 &
  19.651 &
  \multicolumn{1}{c|}{0.737} &
  0.059 &
  24.627 &
  \multicolumn{1}{c|}{0.762} &
  0.078 &
  22.203 &
  \multicolumn{1}{c|}{0.757} &
  0.057 &
  24.833 &
  \multicolumn{1}{c|}{0.743} &
  0.076 &
  22.360 &
  0.767 \\
bust &
  0.106 &
  19.511 &
  \multicolumn{1}{c|}{0.459} &
  0.078 &
  22.174 &
  \multicolumn{1}{c|}{0.829} &
  0.120 &
  18.417 &
  \multicolumn{1}{c|}{0.818} &
  0.094 &
  20.513 &
  \multicolumn{1}{c|}{0.809} &
  0.084 &
  21.486 &
  \multicolumn{1}{c|}{0.823} &
  0.076 &
  22.414 &
  \multicolumn{1}{c|}{0.790} &
  0.093 &
  20.629 &
  0.819 \\
einstein &
  0.065 &
  23.752 &
  \multicolumn{1}{c|}{0.443} &
  0.077 &
  22.240 &
  \multicolumn{1}{c|}{0.788} &
  0.068 &
  23.347 &
  \multicolumn{1}{c|}{0.874} &
  0.051 &
  25.819 &
  \multicolumn{1}{c|}{0.881} &
  0.076 &
  22.392 &
  \multicolumn{1}{c|}{0.857} &
  0.064 &
  23.874 &
  \multicolumn{1}{c|}{0.836} &
  0.076 &
  22.412 &
  0.856 \\
soap &
  0.120 &
  18.416 &
  \multicolumn{1}{c|}{0.301} &
  0.108 &
  19.336 &
  \multicolumn{1}{c|}{0.501} &
  0.140 &
  17.096 &
  \multicolumn{1}{c|}{0.757} &
  0.103 &
  19.772 &
  \multicolumn{1}{c|}{0.775} &
  0.077 &
  22.326 &
  \multicolumn{1}{c|}{0.768} &
  0.066 &
  23.577 &
  \multicolumn{1}{c|}{0.780} &
  0.086 &
  21.355 &
  0.732 \\ \hline
average &
  0.086 &
  21.535 &
  \multicolumn{1}{c|}{0.456} &
  0.082 &
  21.835 &
  \multicolumn{1}{c|}{0.700} &
  0.100 &
  20.312 &
  \multicolumn{1}{c|}{0.795} &
  0.071 &
  23.263 &
  \multicolumn{1}{c|}{0.815} &
  0.076 &
  22.463 &
  \multicolumn{1}{c|}{0.799} &
  0.070 &
  23.181 &
  \multicolumn{1}{c|}{0.775} &
  0.079 &
  22.107 &
  0.798 \\ \hline
\end{tabular}

\end{minipage}

\end{sidewaystable}
